# Supplementary material for: JADES: Differing assembly histories of galaxies -- Observational evidence for bursty SFHs and (mini-)quenching in the first billion years of the Universe
Source: arXiv:2306.02470 source file (2023-06-08)
Supplement: Supplementary file 1 [file supplement.tex]

\section{Supplementary material [not for submission]}
This section contains material not for submission, but for internal review only.

\subsection{Sample selection [not for submission]}
